# Supplementary material for: Space-time smoothing models for sub-national measles routine immunization coverage estimation with complex survey data
Source: arXiv:2007.03732 ancillary file (2020-07-07)
Supplement: Supplementary file 1 [file SuppInfo.pdf]

# SUPPLEMENT TO "SPACE-TIME SMOOTHING MODELS FOR SUB-NATIONAL MEASLES ROUTINE IMMUNIZATION COVERAGE ESTIMATION WITH COMPLEX SURVEY DATA"

BY TRACY QI DONG[1,*] AND JON WAKEFIELD[1,2]

[1]Department of Biostatistics, University of Washington [*]qd8@uw.edu

[2]Department of Statistics, University of Washington

## S1. Models for structured spatial/temporal random effects.

S1.1. *Intrinsic conditional autoregressive (ICAR) model.* The intrinsic conditional autoregressive (ICAR) model is an intrinsic Gaussian Markov random field (IGMRF) with the density

$$\pi(\boldsymbol{x}|\kappa) \propto \kappa^{(rank(\boldsymbol{Q})-1)/2} \exp\left(-\frac{1}{2}\boldsymbol{x}^\intercal \boldsymbol{Q}\boldsymbol{x}\right),$$

where $\kappa$ is the precision parameter, and $\boldsymbol{Q} = \kappa\boldsymbol{R}$ is the precision matrix with a structure matrix $\boldsymbol{R}$ with the following elements:

$$R_{ij} = \begin{cases} m_i \; i = j \\ -1 \; i \sim j \\ 0 \quad \text{otherwise} \end{cases}$$

where $m_i$ is the number of neighbors of the $i$th element, and $j \sim i$ means the $j$th element is a neighbor of the $i$th element.

The ICAR model is commonly used for spatial random effects in Bayesian hierarchical models. It can be specified conditionally via

$$x_i|\boldsymbol{x}_{-i}, \kappa \sim \mathrm{N}\left(\frac{1}{m_i}\sum_{j:j\sim i} x_j, \frac{1}{m_i\kappa}\right).$$

S1.2. *Second-order random walk (RW2) model.* The second-order random walk (RW2) model of regular locations is an IGMRF of second order with density

$$\pi(\boldsymbol{x}|\kappa) \propto \kappa^{(n-2)/2} \exp\left(-\frac{1}{2}\boldsymbol{x}^\intercal \boldsymbol{Q}\boldsymbol{x}\right),$$

where $\kappa$ is the precision parameter, and $\boldsymbol{Q} = \kappa\boldsymbol{R}$ is the precision matrix with a structure matrix $\boldsymbol{R}$ of the following form:

$$\boldsymbol{R} = \begin{pmatrix} 1 & -2 & 1 & & & & & & \\ -2 & 5 & -4 & 1 & & & & & \\ 1 & -4 & 6 & -4 & 1 & & & & \\ & 1 & -4 & 6 & -4 & 1 & & & \\ & & \ddots & \ddots & \ddots & \ddots & \ddots & & \\ & & & 1 & -4 & 6 & -4 & 1 & \\ & & & & 1 & -4 & 6 & -4 & 1 \\ & & & & & 1 & -4 & 5 & -2 \\ & & & & & & 1 & -2 & 1 \end{pmatrix}.$$

The RW2 model is commonly used for temporal random effects in Bayesian hierarchical models. It is constructed assuming independent second-order increments

$$\triangle^2 x_i = (x_{i+2} - x_{i+1}) - (x_{i+1} - x_i)|\kappa \sim \mathrm{N}(0, \kappa^{-1}).$$

S1.3. *Autoregressive model of order 1 (AR1) for Gaussian random vectors.* The autoregressive model of order 1 (AR1) for the Gaussian vector $\boldsymbol{x} = [x_1, \ldots, x_n]^\intercal$ is defined as

$$x_1 \sim \mathrm{N}\left(0, \left(\tau(1-\rho^2)\right)^{-1}\right)$$
$$x_i = \rho x_{i-1} + \epsilon_i; \quad \epsilon_i \sim \mathrm{N}\left(0, \tau^{-1}\right) \quad \text{for } i = 2, \ldots, n$$

where $|\rho| < 1$. The marginal precision $\kappa$ is equal to

$$\kappa = \tau(1-\rho^2)$$

Hence, the marginal standard deviation $\sigma$ is equal to

$$\sigma = \kappa^{-1/2} = \left(\tau(1-\rho^2)\right)^{-1/2}$$

**S2. Model assessment metrics.** We briefly describe three model assessment metrics that allow for comparison across a variety of fitted models: the deviance information criteria (DIC), the Watanabe-Akaike information criteria (WAIC) and the log-score conditional predictive ordinate (LCPO).

S2.1. *The deviance information criteria (DIC).* Let $\boldsymbol{\theta}$ be a vector of parameters and $\boldsymbol{y}$ be the observed data, so that $p(\boldsymbol{y}|\boldsymbol{\theta})$ is the data model, $p(\boldsymbol{\theta})$ is the prior and $p(\boldsymbol{\theta}|\boldsymbol{y})$ is the posterior. The *deviance*, which provides a measure of model "mis-fit", is defined as

$$D = -2\log p(\boldsymbol{y}|\boldsymbol{\theta}).$$

Let $\bar{\boldsymbol{\theta}} = \mathbb{E}\left[\boldsymbol{\theta}|\boldsymbol{y}\right]$ be the posterior mean. The *effective number of parameters*, which provides a measure of model complexity, is defined as

$$p_{DIC} = \mathbb{E}_{\boldsymbol{\theta}}\left[D|\boldsymbol{y}\right] - D(\bar{\boldsymbol{\theta}}),$$

where $\mathbb{E}_{\boldsymbol{\theta}}\left[D|\boldsymbol{y}\right]$ represents the posterior mean of the *deviance*, and $D(\bar{\boldsymbol{\theta}})$ represents the *deviance* evaluated at the posterior mean $\bar{\boldsymbol{\theta}}$. The DIC is then defined as

$$\begin{aligned} DIC &= p_{DIC} + \mathbb{E}_{\boldsymbol{\theta}}\left[D|\boldsymbol{y}\right] \\ &= 2\mathbb{E}_{\boldsymbol{\theta}}\left[D|\boldsymbol{y}\right] - D(\bar{\boldsymbol{\theta}}) \\ &= 2p_{DIC} + D(\bar{\boldsymbol{\theta}}) \end{aligned}$$

Therefore, a lower DIC value generally indicates a better model fit.

The DIC can be viewed as a hierarchical modeling generalization of the Akaike information criterion (AIC) and Bayesian information criterion (BIC). It is based on asymptotic arguments and may under-penalize complex models with many random effects (Spiegelhalter et al., 2014).

S2.2. *The Watanabe-Akaike information criteria (WAIC).* The WAIC, also known as the *widely applicable information criterion*, was first described in Watanabe (2010) and has been receiving increasing popularity. It is a fully Bayesian approach for estimating the out-of-sample expectation, starting with the computed *log point-wise posterior predictive density* and then adding a correction for *effective number of parameters* to adjust for overfitting (Gelman, Hwang and Vehtari, 2014). Specifically, the *log point-wise posterior predictive density* is defined as

$$\sum_i \log p(y_i|\boldsymbol{y}) = \sum_i \log \int p(y_i|\boldsymbol{\theta})p(\boldsymbol{\theta}|\boldsymbol{y})d\boldsymbol{\theta},$$

and the *effective number of parameters* is defined as

$$p_{WAIC} = \sum_i \log \mathbb{E}\left[p(y_i|\boldsymbol{\theta})|\boldsymbol{y}\right] - \mathbb{E}\left[\log p(y_i|\boldsymbol{\theta})|\boldsymbol{y}\right].$$

The WAIC is then defined as

$$WAIC = 2p_{WAIC} - 2\sum_i \log p(y_i|\boldsymbol{y})$$

Therefore, a lower WAIC value generally indicates a better model fit.

Compared to the DIC, the WAIC utilizes the whole posterior distribution, instead of just the posterior mean. It can be computed using posterior samples.

S2.3. *The log-score conditional predictive ordinate (LCPO).* The conditional predictive ordinate (CPO) is a leave-one-out cross-validation score. It is defined as

$$\text{CPO}_i = p(y_i|\boldsymbol{y}_{-i}),$$

where $\boldsymbol{y}_{-i}$ denotes the observations $\boldsymbol{y}$ with the $i$th component removed. It represents the posterior probability of observing $y_i$ when the model is fitted to all other data. Therefore, a higher value of CPO generally indicates a better fit of the model to $y_i$, and a low value suggest that $y_i$ is an outlier or influential observation.

The log-score CPO (LCPO) is defined as

$$\text{LCPO} = -\frac{1}{n}\sum_i^n \log \text{CPO}_i$$

The negative sign is added here so that a smaller value of the LCPO indicates a better prediction quality of the model, which is consistent with DIC and WAIC.

## S3. Summary information of household surveys and SIAs.

TABLE S1

*Summary information of survey sampling design, including source of sampling frame, survey strata, cluster and household sample sizes, age group with vaccination data, and features of weight calculation.*

| Survey Time | Survey Type | Census from which Sampling Frame is derived | Strata | #Clusters per State | #Households per Cluster | Age Group with Vaccination Data | Base Weight Calculated using Stage 1 & 2 Selection Probabilities | Non-response Adjustment | Post-stratification |
|---|---|---|---|---|---|---|---|---|---|
| Mar. – Aug. 2003 | DHS | 1991 | Urban/Rural within State | 2–21 | 19–24 | 0 – 59 months | ✓ | ✓ | |
| Mar. – Apr. 2007 | MICS | 1991 | State | 30 | 25 | 0 – 59 months | ✓ | ✓ | |
| Jun. – Oct. 2008 | DHS | 2006 | Urban/Rural within State | 23–32 | 41 | 0 – 59 months | ✓ | ✓ | |
| Feb. – Mar. 2011 | MICS | 2006 | State | 40 | 20 | 0 – 59 months | ✓ | ✓ | |
| Feb. – Jun. 2013 | DHS | 2006 | Urban/Rural within State | 25–40 | 45 | 0 – 59 months | ✓ | ✓ | |
| Feb. – May 2014 | NNHS | 2006 | State | 30–35 | 22 | 0 – 59 months | | | ✓ |
| Jul. – Sep. 2015 | NNHS | 2006 | State | 32 | 22 | 0 – 59 months | | | ✓ |
| Sep. 2016 – Feb. 2017 | MICS/NICS | 2006 | State | 60–120 | 16 | 0 – 35 months | ✓ | ✓ | |
| Aug. – Dec. 2018 | DHS | 2006 | Urban/Rural within State | 35–53 | 30 | 0 – 35 months | ✓ | ✓ | |

TABLE S2

*The start and end dates, target age groups, and geographical areas of the SIAs in Nigeria we use for the analysis. There are 20 northern states and 17 southern states in Nigeria.*

| Start Date | End Date | Target Age Group | Geographic Areas |
|---|---|---|---|
| 12/06/2005 | 12/10/2005 | 9M–15Y | Northern States |
| 10/03/2006 | 10/09/2006 | 9M–15Y | Southern States |
| 11/26/2008 | 12/15/2008 | 9–59M | All States |
| 01/26/2011 | 01/30/2011 | 9–59M | Northern States |
| 02/23/2011 | 02/27/2011 | 9–59M | Southern States |
| 10/05/2013 | 10/09/2013 | 9–59M | Northern States |
| 11/02/2013 | 11/25/2013 | 9–59M | Southern States |
| 12/21/2015 | 11/25/2015 | 9M–10Y | Northern States |
| 01/28/2016 | 02/01/2016 | 9–59M | Southern States |
| 11/09/2017 | 11/30/2017 | 9–59M | Northern States |
| 03/01/2018 | 03/30/2018 | 9–59M | Southern States |

**S4. Simulation study.** We conduct a simulation study to examine how our approach performs under a number of scenarios with surveys of various sizes. Under each scenario, we compare two models:

1. *RI+SIA Model*: this model is similar to that described by Equations (1) – (3) in Section 3.3 of the main paper, but omitting the survey-specific effects, i.e. $\theta_{ibs} = \mu_{ib} + \beta_1 \times x_{ibs}$. For RI-specific coverage estimation, this model will be applied to the simulated survey data from birth cohorts that either had RI only or had RI plus one SIA opportunity.
2. *RI Only Model*: this model is similar to the *RI+SIA Model*, but omitting the component accounting for the impact of SIA, i.e., $\theta_{ibs} = \mu_{ib}$. This model will be applied to the simulated survey data from birth cohorts that had RI only — the same as the current common practice for RI-specific coverage estimation.

S4.1. *Set up.* We simulate complete enumeration areas (EAs) and households within each of Nigeria's 37 states based on the distribution of population and EAs summarized in Table B.1 in the 2013 Nigeria DHS report (National Population Commission - NPC and ICF, 2014). For faster computation, the number of simulated EAs in each state is set to be one tenth of the true number of EAs, and each EA has 80 simulated households.

A total of 34 birth cohorts of children born between 2000 and 2016 are simulated assuming 1 new live birth per EA per month — a rate similar to Nigeria's birth rate during that time period (The World Bank, 2019). Each simulated child is randomly assigned to a household. The resultant population from this step is used for the entire simulation study.

Next, for each iteration, we simulate RI and SIA activities roughly based on what have been implemented in Nigeria between 2000 and 2016. All children have their RI opportunities at the age of 9 months. In addition, we take Jan. 2000 as month 1 and let there be five SIAs conducted in all states in months 72, 108, 134, 167 and 193 respectively. We simulate the true RI-specific MCV1 coverage for children in birth cohort $b$ in state $i$, $p_{\text{RI},ib}$, and the increase in the overall MCV1 coverage by the first SIA opportunity, $q_{\text{SIA},ib}$, under the following model:

$$\begin{aligned}
p_{\text{RI},ib} &= \text{expit}(\beta_0 + \alpha_i + \gamma_i + \delta_b + \tau_b + \phi_{ib}) \\
&= \text{expit}(\mu_{ib}) \\
q_{\text{SIA},ib} &= \text{expit}(\mu_{ib} + \beta_1) - \text{expit}(\mu_{ib}) \\
&= \text{expit}(\mu_{ib} + \beta_1) - p_{\text{RI},ib}
\end{aligned}$$

$$\begin{gathered}
\alpha_i \sim \text{ICAR}(\sigma_\alpha) \quad \gamma_i \sim_{iid} \text{Normal}(0, \sigma_\gamma) \\
\delta_b \sim \text{RW2}(\sigma_\delta) \quad \tau_b \sim_{iid} \text{Normal}(0, \sigma_\tau) \\
\phi_{ib} \sim_{iid} \text{Normal}(0, \sigma_\phi)
\end{gathered}$$

The true values for the parameters are specified as follows:

$$\begin{gathered}
\beta_0 = 0 \quad \beta_1 = 0.8 \\
\sigma_\alpha = 0.8 \quad \sigma_\gamma = 0.01 \\
\sigma_\delta = 0.8 \quad \sigma_\tau = 0.01 \\
\sigma_\phi = 0.2
\end{gathered}$$

The MCV1 status for each child over time is simulated based on the true RI and SIA coverage in the birth cohort and state that the child belongs to.

A total of eight surveys are simulated based on the survey schedule in Nigeria between 2000 and 2017. Each survey is stratified by state and adopts a two-stage cluster sampling

design. No stratification by urban/rural is carried out in this simulation study. Within each state $i$ (i.e., stratum), $c_i$ clusters are randomly sampled from the $C_i$ EAs in the first stage, then within each selected cluster, $h_{ic}$ households are randomly sampled from the $H_{ic}$ households in the second stage. All children under 5 years of age in the selected households are sampled, and their MCV1 status are recorded.

Using the simulated survey data, we implement the data processing and design-based coverage estimation procedures described in Section 3 of the main paper. We then apply the *RI+SIA Model* and *RI Only Model* to the respective data sets to obtain the point estimates and associated 95% posterior credible intervals of the state-level RI-specific MCV1 coverage for each birth cohort.

The performance of our approach is examined under a number of scenarios with surveys of various sizes. Specifically, we conduct 300 iterations under each combination of $c_i = 20, 40, 60$ and $h_{ic} = 15, 30, 45$, with each iteration using a different simulated data set. The estimation accuracy and precision of the two models are evaluated based on four metrics: bias, RMSE, the nominal coverage and the average widths of 95% posterior CIs of the estimated RI-specific coverage $p_{\text{RI},ib}$ across all areas and birth cohorts.

S4.2. *Results.* The simulation results are summarized in Figure S1. In each plot, results from the *RI+SIA Model* and *RI Only Model* are represented by red and blue dots respectively, with darker shades corresponding to greater numbers of households sampled per cluster. Along the x-axis from left to right are increasing numbers of clusters sampled per state.

Both models have very small bias under all scenarios. Within each model, both the RMSE and the 95% nominal coverage improves as the number of clusters per state and the number of households per cluster increases. The average CI widths show a similar trend in general, except for when the *RI Only Model* is applied to very sparse data ($c_i = 20, h_{ic} = 15$).

Under each scenario, the *RI+SIA Model* always outperforms the *RI Only Model* in terms of RMSE, coverage and average CI widths. This demonstrates the improved accuracy and precision of the RI-specific coverage estimation by the *RI+SIA Model*, which makes more efficient use of data by having a model component that accounts for the impact of SIAs and incorporating information from birth cohorts who had an SIA opportunity in addition to RI.

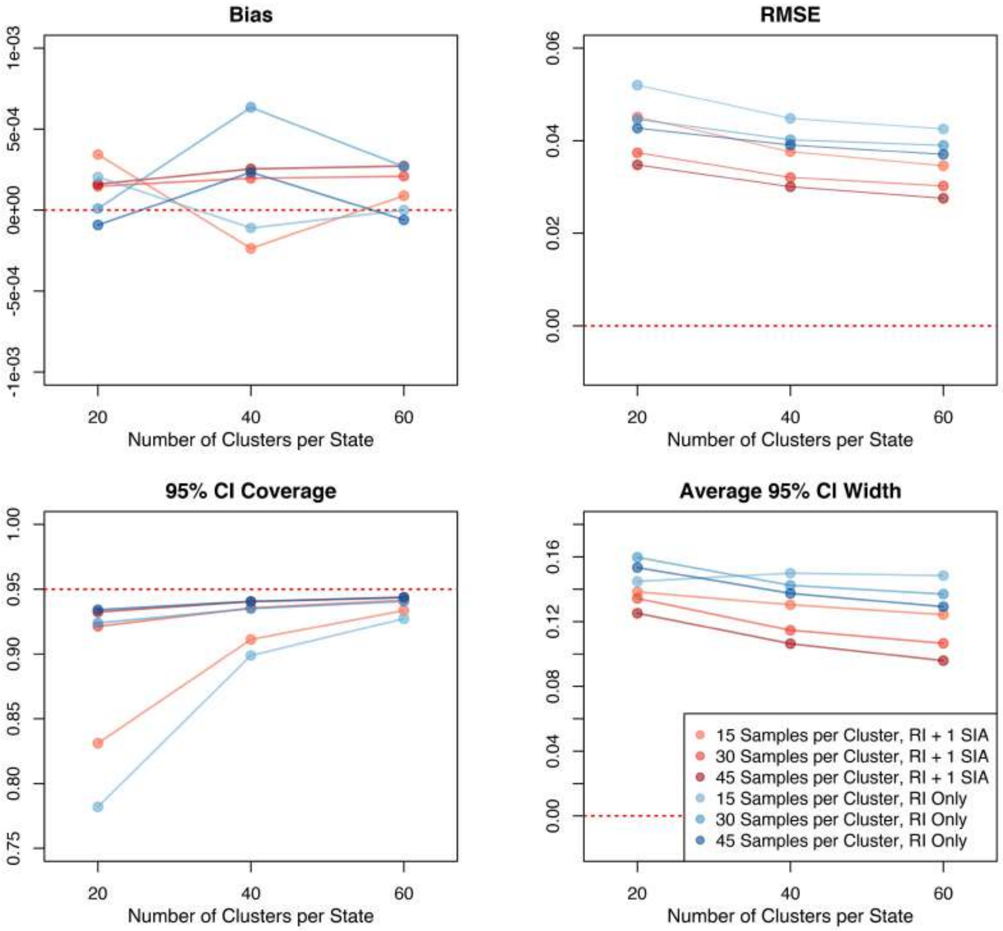


FIG S1. *Summary results of the simulation study, including bias, root mean square error (RMSE), the nominal coverage and the average widths of 95% posterior credible intervals (CIs) of the estimated RI-specific MCV1 coverage $p_{RI,ib}$ across all areas and birth cohorts.*

## S5. Tables and plots for the sensitivity analysis using 12-month birth cohorts.

TABLE S3
*Summary of model assessment metrics and parameter estimates in the sensitivity analysis with 12-month birth cohort data. Bold figures represent the "best" models according to the relevant criteria. The posterior medians are taken as the point estimates and the corresponding posterior 95% CIs are shown in the parentheses.*

| | Model Assessment Metric | | | Parameter Estimate | | | | | | | | |
|---|---|---|---|---|---|---|---|---|---|---|---|---|
| Model | DIC | WAIC | LCPO | Intercept $\beta_0$ | SIA $\beta_1$ | ICAR $\sigma_\alpha$ | Area IID $\sigma_\gamma$ | RW2 $\sigma_\delta$ | Time IID $\sigma_\tau$ | Space×Time $\sigma_\phi$ | Survey $\sigma_\epsilon$ | AR1 $\rho_\phi$ |
| IID-IID | 1333 | 1463 | 1.112 | 0.211 (-0.019, 0.460) | 0.195 (0.013, 0.368) | 0.66 (0.52, 0.85) | 0.071 (0.010, 0.238) | 0.072 (0.007, 0.362) | 0.081 (0.026, 0.193) | 0.37 (0.33, 0.41) | 0.21 (0.12, 0.40) | |
| ICAR-IID | 1319 | 1452 | 1.078 | 0.206 (-0.029, 0.456) | 0.198 (0.012, 0.376) | 0.66 (0.52, 0.86) | 0.075 (0.010, 0.245) | 0.077 (0.008, 0.382) | 0.105 (0.049, 0.212) | 0.38 (0.33, 0.43) | 0.20 (0.11, 0.39) | |
| IID-RW2 | 1294 | 1401 | 1.007 | 0.225 (-0.019, 0.468) | 0.173 (-0.020, 0.358) | 0.288 (0.028, 1.487) | 0.184 (0.026, 0.964) | 0.107 (0.014, 0.537) | 0.126 (0.066, 0.235) | 0.40 (0.31, 0.51) | 0.20 (0.11, 0.39) | |
| ICAR-RW2 | 1281 | 1387 | 0.991 | 0.227 (-0.031, 0.503) | 0.162 (-0.028, 0.344) | 0.283 (0.027, 1.453) | 0.144 (0.014, 0.736) | 0.078 (0.008, 0.397) | 0.125 (0.064, 0.235) | 0.43 (0.34, 0.55) | 0.20 (0.12, 0.40) | |
| IID-AR1 | 1273 | 1387 | 1.018 | 0.227 (-0.024, 0.496) | 0.168 (-0.017, 0.347) | 0.60 (0.45, 0.81) | 0.068 (0.009, 0.238) | 0.078 (0.008, 0.388) | 0.104 (0.045, 0.211) | 0.46 (0.38, 0.56) | 0.21 (0.12, 0.40) | 0.81 (0.70, 0.89) |
| ICAR-AR1 | **1264** | **1377** | **0.994** | 0.220 (-0.013, 0.474) | 0.176 (-0.011, 0.353) | 0.47 (0.28, 0.71 | 0.073 (0.010, 0.238) | 0.077 (0.008, 0.385) | 0.103 (0.047, 0.214) | 0.58 (0.44, 0.83) | 0.21 (0.12, 0.40) | 0.88 (0.78, 0.95) |

TABLE S4
*Proportions of variance explained by each random effect component (percent) in the sensitivity analysis with 12-month birth cohort data.*

| Model | ICAR $\sigma^2_\alpha$ | Space IID $\sigma^2_\gamma$ | RW2 $\sigma^2_\delta$ | Time IID $\sigma^2_\tau$ | Space×Time $\sigma^2_\phi$ | Survey $\sigma^2_\epsilon$ |
|---|---|---|---|---|---|---|
| IID-IID | 81.5 | 1.4 | 3.1 | 0.7 | 10.0 | 3.3 |
| ICAR-IID | 80.2 | 1.7 | 3.1 | 0.9 | 11.0 | 3.2 |
| IID-RW2 | 23.9 | 9.8 | 3.3 | 4.6 | 46.6 | 11.7 |
| ICAR-RW2 | 17.0 | 4.0 | 1.6 | 0.6 | 75.1 | 1.8 |
| IID-AR1 | 74.4 | 1.4 | 3.2 | 0.9 | 16.6 | 3.5 |
| ICAR-AR1 | 43.0 | 1.9 | 3.8 | 1.1 | 45.8 | 4.4 |

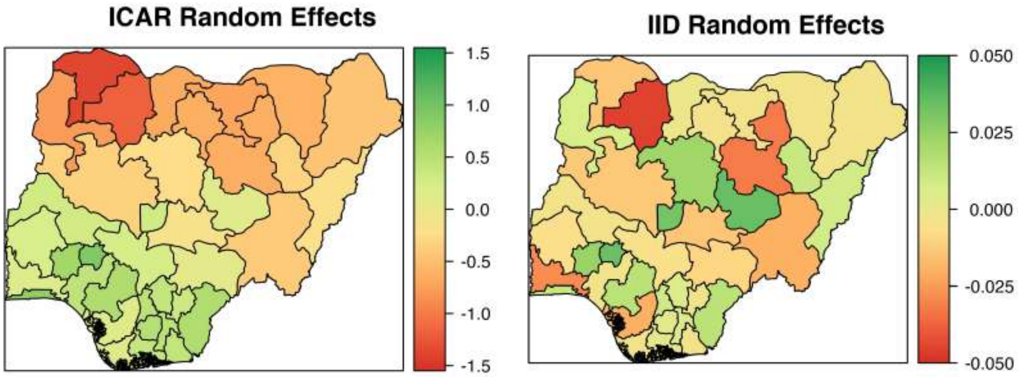


FIG S2. *The posterior medians of the ICAR spatial random effects $\alpha_i$ (left) and the IID random effects $\gamma_i$ (right) from the fitted ICAR-AR1 Model in the sensitivity analysis with 12-month birth cohort data.*

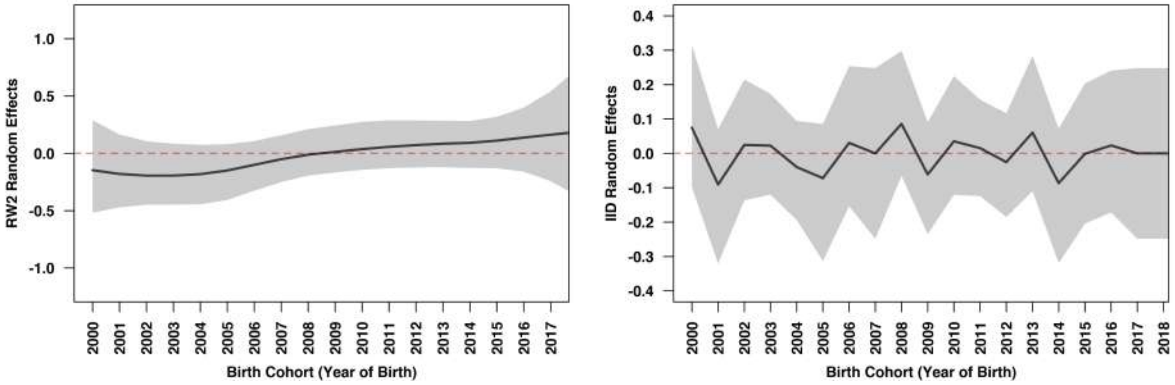


FIG S3. *The posterior medians and 95% CIs of the RW2 temporal random effects $\delta_b$ (left) and the IID random effects $\tau_b$ (right) from the fitted ICAR-AR1 Model in the sensitivity analysis with 12-month birth cohort data.*

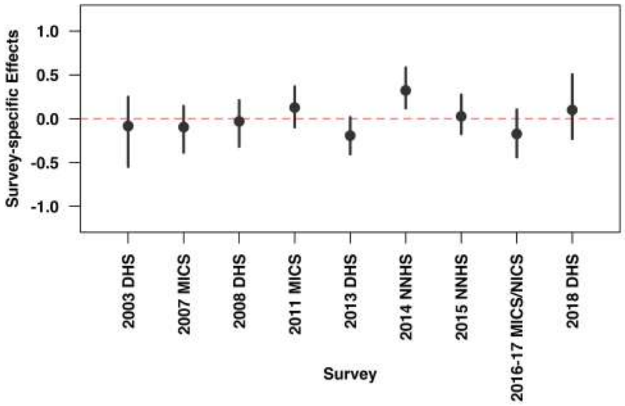


FIG S4. *The posterior medians and 95% CIs of the independent survey-specific effects $\epsilon_s$ in the sensitivity analysis with 12-month birth cohort data..*

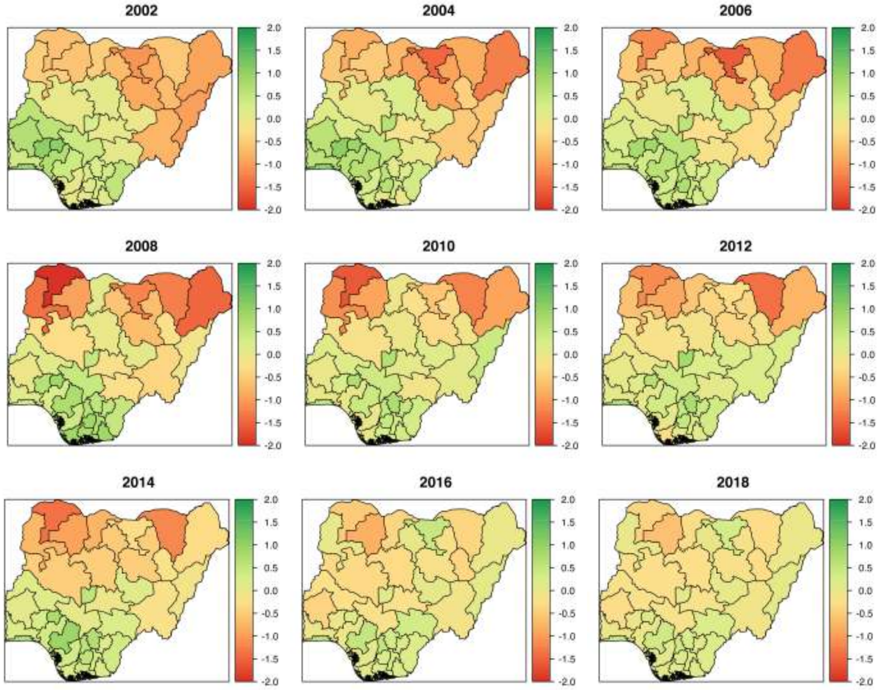


FIG S5. *The posterior medians of the space-time interactions $\phi_{ib}$ across space over selected 12-month birth cohorts from the fitted ICAR-AR1 Model in the sensitivity analysis. Specifically, each map shows the estimated interaction for the cohorts born in the corresponding year.*

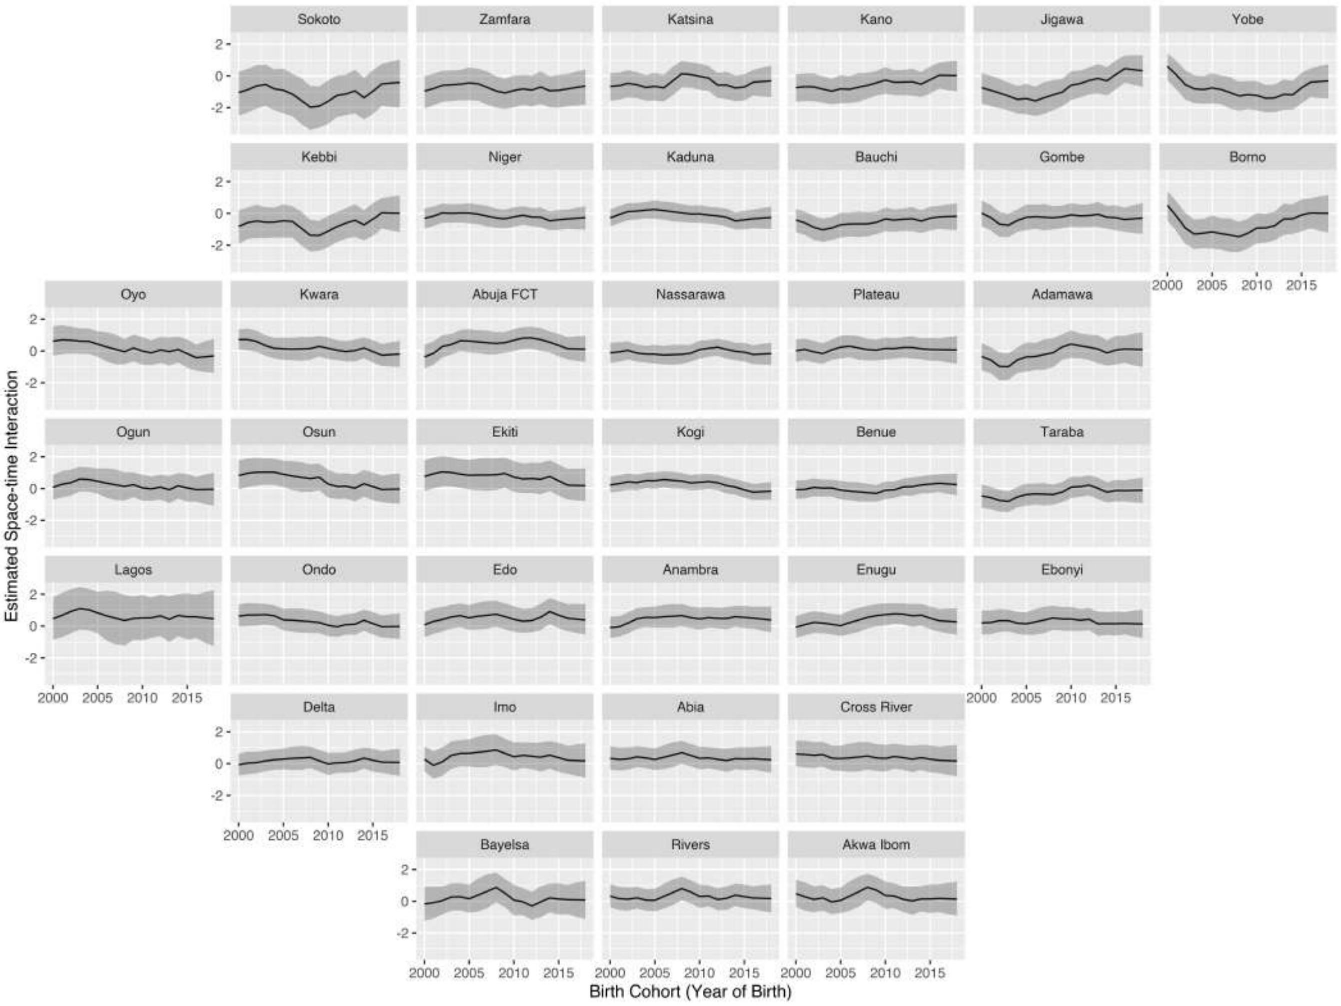


FIG S6. *The posterior medians of the space-time interactions $\phi_{ib}$ over time in all states from the fitted ICAR-AR1 Model in the sensitivity analysis with 12-month birth cohort data.*

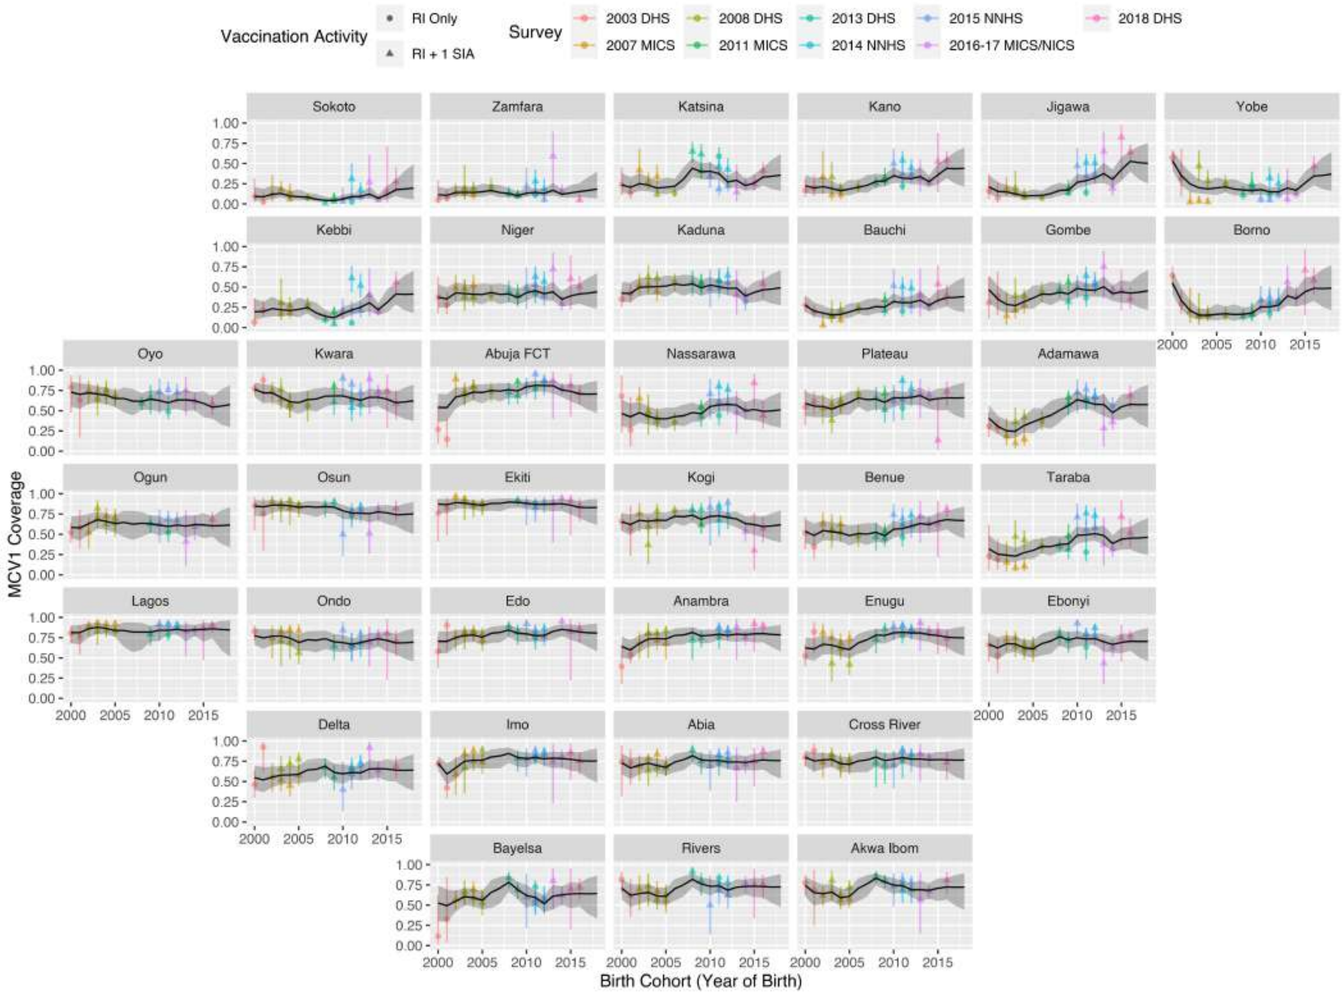


FIG S7. *The posterior medians of the state-level RI-specific MCV1 coverage (dark grey lines) and the associated 95% CIs (light grey ribbons) for the 12-month birth cohorts born between 2000 and 2018 based on the fitted ICAR-AR1 Model in the sensitivity analysis. The design-based overall MCV1 coverage estimates were also shown for references.*

## REFERENCES

THE WORLD BANK (2019). The World Bank DataBank. https://databank.worldbank.org/data/home.aspx.

GELMAN, A., HWANG, J. and VEHTARI, A. (2014). Understanding predictive information criteria for Bayesian models. *Statistics and Computing* **24** 997–1016.

NATIONAL POPULATION COMMISSION - NPC AND ICF (2014). Nigeria Demographic and Health Survey 2013 - Final Report. Abuja, Nigeria: NPC and ICF. Available at http://dhsprogram.com/pubs/pdf/FR293/FR293.pdf.

SPIEGELHALTER, D. J., BEST, N. G., CARLIN, B. P. and VAN DER LINDE, A. (2014). The deviance information criterion: 12 years on. *Journal of the Royal Statistical Society: Series B (Statistical Methodology)* **76** 485–493.

WATANABE, S. (2010). Asymptotic equivalence of Bayes cross validation and widely applicable information criterion in singular learning theory. *Journal of Machine Learning Research* **11** 3571–3594.
